# Supplementary material for: OG-Mapping: Octree-based Structured 3D Gaussians for Online Dense Mapping
Source: arXiv:2408.17223 source file (2024-08-30)
Supplement: Supplementary file 1 [file X_suppl.tex]

\clearpage
\setcounter{page}{1}
\maketitlesupplementary

\section{Implementation Details}
{
  \label{sec:Implementation Details}
  In this section, we report the detailed settings and hyperparameters used in OG-Mapping. 
  
  {
  \noindent
  \textbf{Anchors Feature Encoding.}
  {
    There are various possible methods for encoding $f_v$,  and it is essential to explore the different impacts of these encoding techniques.
    we evaluated three different encoding function $encoding(.)$ to $f_v$: (1) Two Hash Grids, (2) Single Hash Grid and (3) w/o Hash Grid. 
    For the first encoding method, we utilized two separate multi-resolution hash-based feature grid (one for $\textbf{F}_{color}$ and the other for $\textbf{F}_{opacity}$ and $\textbf{F}_{cov}$ ).
    The spatial resolution of each level ranges from the coarsest $R_{min}=16$ to the finest $R_{max}$ with a total of 16 levels, where the $R_{max}$ is determined by the voxel size of the coarsest granularity level of anchors.
    For the second encoding method, we employ only single hash grid with the same parameter settings as the first.
    In terms of the final encoding method, each anchor is equipped with a local context feature consisting of $(f_{color}, f_{opacity}, f_{cov})$, where $f_{color}$ has a dimension of 16, and both $f_{opacity}$ and $f_{cov}$ have dimensions of 8.
    
    For Replica, we utilize the first encoding method. For other dataset, we use the final encoding method.
    Specifically, for the sparse versions provided across all datasets, we employed the final encoding method.
    For the analysis of different encoding methods, please refer to Sec. \ref{sec:encoding_analysis}.
  }
  
  \noindent
  \textbf{Feature decoders.}
  {
    The feature decoders($\textbf{F}_{color}, \textbf{F}_{opacity}$ and $ \textbf{F}_{cov}$) are all implemented in a Linear-ReLU-Linear type with 32 hidden dimension. The output feature vector is activated by a head layer. 
    Fig. \ref{fig: decoder} provides an overview of the MLP structure for different encoding functions.
    For color, the output is activated using a $Sigmoid$ function. For rotation, we activate it with a normalization following 3D-GS \cite{3dgs} and Scaffold-GS \cite{scaffoldgs}. For scaling, we adjust the base scaling $s_v$ of anchor $v$ with the decoder output as Scaffold-GS.
    For opacity, we use the Sigmoid function as the activation function instead of the Tanh function used in Scaffold-GS. 
    Since the range of Tanh function is [-1,1], Gaussian kernels may get negative opacity values and will not participate in the differentiable reconstruction process, until the $F_{opacity}$ activates them after many iterations. 
    Therefore, this function is not suitable for online dense mapping, which requires fast inference. In contrast, the Sigmoid activation function ensures all 3D Gaussians have vaild opacity values. We empirically found that the Sigmoid activation function performs better with the same number of iterations.
  } 
  \begin{figure}[thp]
    \begin{center}
    \includegraphics[width=1.0\linewidth]{./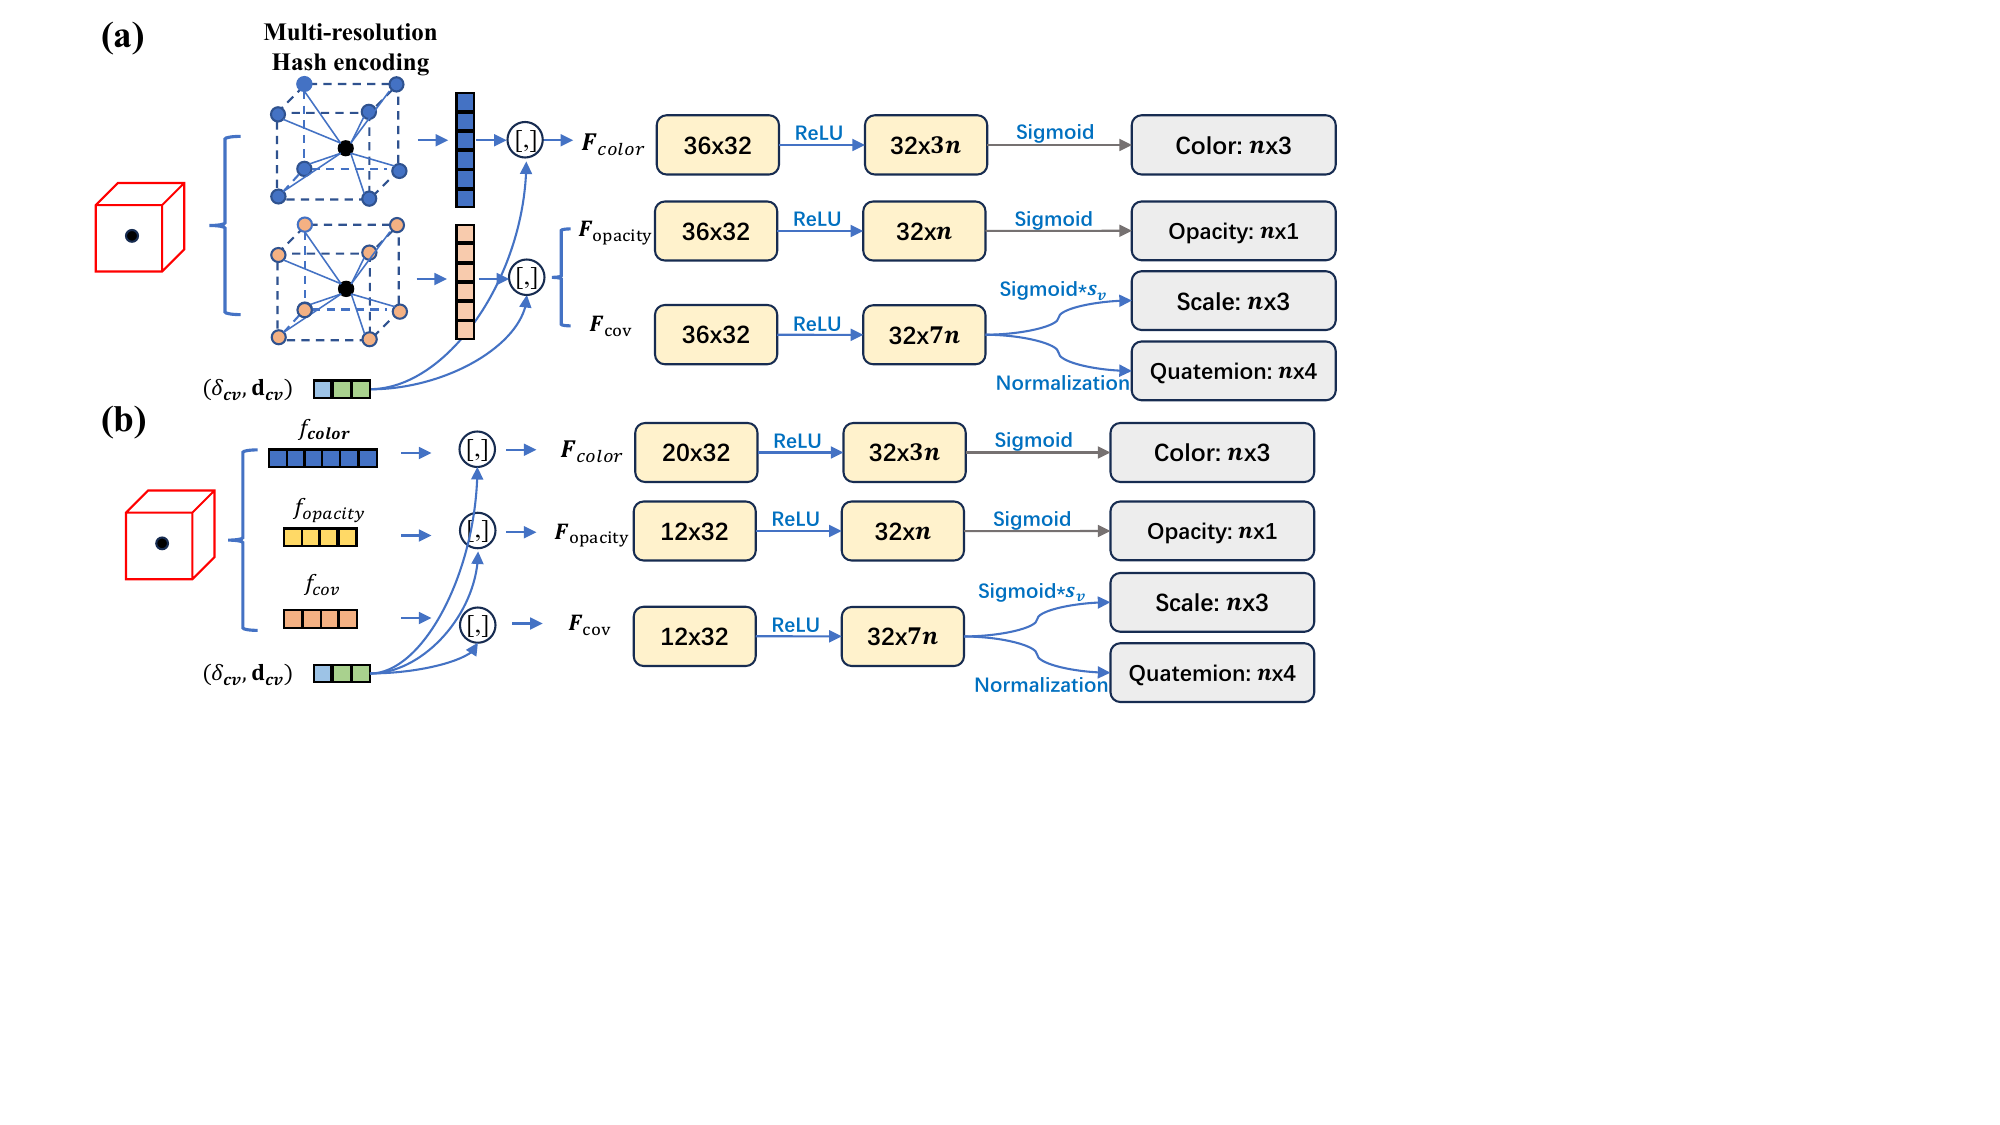}
    \end{center}
       \caption{ MLP structures for (a) Two Hash Grids and (b) w/o Hash Grid. We utilize three small MLPs ($\textbf{F}_{color}, \textbf{F}_{opacity}$ and $\textbf{F}_{cov}$) to predict attributes(color, opacity, scale and quaternion) of $n$ 3D Gaussians. $\delta _{cv}$ represents the distance between the camera and anchor point, and $\textbf{d}_{cv}$ represents the relative direnction. }
    \label{fig: decoder}
  \end{figure}

  \noindent
  \textbf{Hyperparameters setting.}
  {
    For all scenes, we used a maximum of three levels( $l \in \{0, 1, 2\}$).
    We set the dynamic keyframe window size to 10 and employ 6 iterations for bundle adjustment. 
    For the training of our scene representation, we use learning rate of 0.008, 0.002 and 0.004 for $\textbf{F}_{color}, \textbf{F}_{opacity}$ and $\textbf{F}_{cov}$, respectively. We matain $\tau_0$ at a constant 0.0002. 
    The number of learnable offsets $n$ is set to 5.
    The weights of each loss are $\lambda_{c}=0.8,\lambda_{SSIM}=0.2,\lambda_{d}=0.5, \lambda_{s}=0.01$. 
    For the Replica dataset, we use the two hash grad encoding method and the feature learning rate is set to 0.0075. We set the learning rate of Gaussians' offsets to 0.001. The coarsest level voxel size is set to 2.5 cm. In term of the keyframe threshold $\varrho$, the value is set to a constant 0.85.
    For the ScanNet dataset, the coarsest granularity voxel size is set to 4 cm. The learning rate of Gaussians' offsets is also increased to 0.01. We employ the local context encoding method(the w/o Hash Grid introduced in above part) with 0.0075 as the learning rate. The $\varrho$ is set to a constant 0.75.
  }
  }
}
\section{Experiments and Results}
{
\noindent
\textbf{Opacity activation function analysis.}
{
  We conducted experimental validation on the Scannet and Replica datasets to analyze the effects of the Tanh and Sigmoid activation functions on $\textbf{F}_{opacity}$.
  The comparison results are shown in Tab. \ref{tab: activation}.
  The results indicate that under the same conditions, the Sigmoid activation function performs better.
}

\begin{table}[h]
  %\centering
  \resizebox{\linewidth}{!}{
      \begin{tabular}{c|ccccc}
          \hline
          \textbf{Dataset}                                  & Methods                            & PSNR                  & SSIM    & LPIPS & \makecell{Model \\Size(MB)}  \\
          \hline
          \multirow{2}{*}{room0}                            & Tanh                               & 35.38                 & 0.965   & 0.056 & 59.1              \\
          \cline{2-6}
                                                            & Sigmoid                            & \textbf{36.24}        & \textbf{0.969}   & \textbf{0.044} & \textbf{39.9}                 \\
                                                              
          \hline
          \multirow{2}{*}{scene0000}                        & Tanh                               & 25.15                 & 0.789   & 0.405 & 59.8                     \\
          \cline{2-6}
                                                            & Sigmoid                            & \textbf{25.81}                 & \textbf{0.807}   & \textbf{0.345} & \textbf{36.9}                  \\
          \hline
          \end{tabular}
  }
  
  \caption{Comparison between different activation function used in opacity of anchor growing methods on room0 of Replica \cite{replica} dataset and scene0000 of ScanNet \cite{scannet} dataset.}
  \label{tab: activation}
\end{table}

\noindent
\textbf{Encoding analysis}
\label{sec:encoding_analysis}
{
  We evaluate our OG-Mapping on the Replica dataset and ScanNet dataset with different anchor feature encoding methods.
  The results are shown in Tab. \ref{tab:performance_comparison} and Fig. \ref{fig: encoding_statis_scannet}.
  
  \begin{figure}[thp]
    \begin{center}
    \includegraphics[width=1.02\linewidth]{./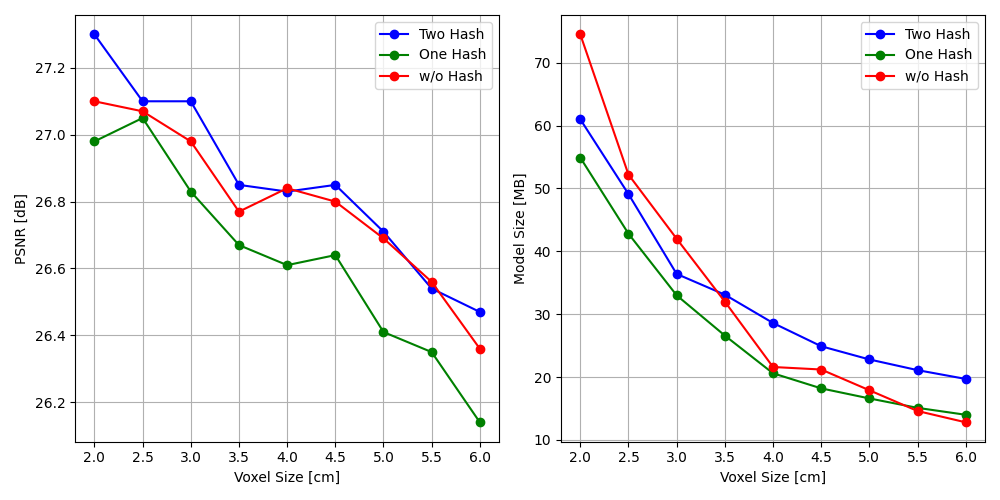}
    \end{center}
       \caption{ The comparative experimental results on scene0169 with different encodings and initial voxel sizes..}
    \label{fig: encoding_statis_scannet}
  \end{figure}
  \begin{table}[h]
    \resizebox{\linewidth}{!}{
    \begin{tabular}{c|cccccc}
        \toprule
        Type&\multicolumn{1}{c}{Method}  & \multirow{1}{*}{PSNR$\uparrow$} & \multirow{1}{*}{SSIM$\uparrow$} & \multirow{1}{*}{LPIPS$\downarrow$}\\
    
        \hline
        \multirow{3}{*}{\makecell{Fixed \\Window}} & Random \cite{eslam}             & 22.54   &   0.797  &  0.275 \\
        \cline{2-5}
        %\hline
        & Overlap \cite{splatam,monogs}     & 22.05   &   0.787  &  0.282 \\
        \cline{2-5}
        %\hline
        & \makecell{Coverage-\\Maximizing \cite{h2mapping}}     & 21.63   &   0.776  &  0.302 \\
        \hline
        \makecell{Dynamic \\Window}& Global(ours)             & \textbf{24.04}   &   \textbf{0.836}  &  \textbf{0.270}\\
        \bottomrule
    \end{tabular}
    }
    \caption{Comparison results of different keyframe window methods on scene0059 \cite{replica}.}
    \label{tab:keyframe_performance_comparison2}
  \end{table}
  \begin{table*}[h]
      \resizebox{\linewidth}{!}{
      \begin{tabular}{c|cccccccccc}
          \toprule
          \multirow{2}{*}{Dataset} & \multicolumn{3}{c}{Anchor Feature Encoding} & \multirow{2}{*}{\makecell{Sparse}} & \multirow{2}{*}{PSNR} & \multirow{2}{*}{\makecell{Mapping/iter\\(ms)}} & \multirow{2}{*}{\makecell{Model Size\\(MB)}} & \multirow{2}{*}{\makecell{Rendering \\FPS}}\\
          \cmidrule(r){2-4}  
           & \makecell{w/o Hash Grid} & \makecell{Single Hash Grid} & \makecell{Two Hash Grids} & & & \\
          \hline
          \multirow{6}{*}{Replica}
            &\checkmark &              &            &            & 38.57     & 13.07   & 50.9  &  489\\
            &           &   \checkmark &            &            & 38.41     & 14.10   & 27.6  &  477\\
            &           &              &  \checkmark&            & 38.56     & 14.53   & 34.6  &  443\\
            &\checkmark &              &            & \checkmark & 37.00     & 9.68    & 8.1   &  582 \\
            &           &   \checkmark &            & \checkmark & 37.78     & 11.08   & 14.6  &  556\\
            &           &              &  \checkmark& \checkmark & 37.89     & 11.12   & 21.3  &  535\\
    
            \bottomrule
      \end{tabular}
      }
      \caption{Comparison of different anchor feature encoding method and pruning setting on Replica dataset.}
      \label{tab:performance_comparison}
  \end{table*}

  The experimental results in Tab. \ref{tab:performance_comparison} indicate that the rendering results using hash grids and local context encoding do not differ significantly. 
  However, the interpolation operations in the hash grids introduce additional computational overhead, resulting in relatively slower runtime and rendering speeds. Despite this, hash grids offer a significant advantage in terms of model storage space.
  We further analyzed the performance of various encodings under different initial voxel sizes. The results are shown in Fig. \ref{fig: encoding_statis_scannet}.
  The results indicate that, in general, smaller initial voxel sizes yield more detailed reconstructed models, but also increase the model's storage space. This outcome is intuitive.
  
  Hash encoding methods transform the encoding problem of individual voxels into a feature encoding problem for the entire scene space. Therefore, they have a more significant advantage in space occupancy, especially in scenarios with denser voxel distributions.
  In addition, as shown in Tab. \ref{tab:performance_comparison}, we conducted experiments to explore the compression effects of pruning on each encoding (i.e., the sparse versions of the data observed in the experiments).
  The scene representation becomes extremely sparse after pruning a large number of anchors. Consequently, the space occupancy of model using local context encoding types is smaller.
  Due to the spatial continuity of hash grid encoding, the opacity distribution of anchors is more uniform, which makes the final impact of pruning relatively minor.
}

\noindent
\textbf{Additional qualitative results on Real-world Scene.}
{
  In our main paper we showed quantitative comparison on the hotel dataset provided by the authors of RTG-SLAM \cite{rtg}. In this section, we show more qualitative results from different views in Fig. \ref{fig: hotel}. As can be seen OG-Mapping achieves better rendering quality.
  In Figure \ref{fig: mesh}, we present the mesh extraction results for SplaTAM \cite{splatam}, RTG-SLAM \cite{rtg}, and our method on the scene0000 and hotel scenes to better showcase the level of details and fidality that OG-Mapping can achieve on those challenging real-world sequences. We render depth maps of every five views and utilize truncated signed distance fusion (TSDF) to fuse the reconstruction depth maps. We set the voxel size to 0.001 and the truncated threshold to 0.04 during TSDF fusion. 
}
\begin{figure}[thp]
  \begin{center}
  \includegraphics[width=0.98\linewidth]{./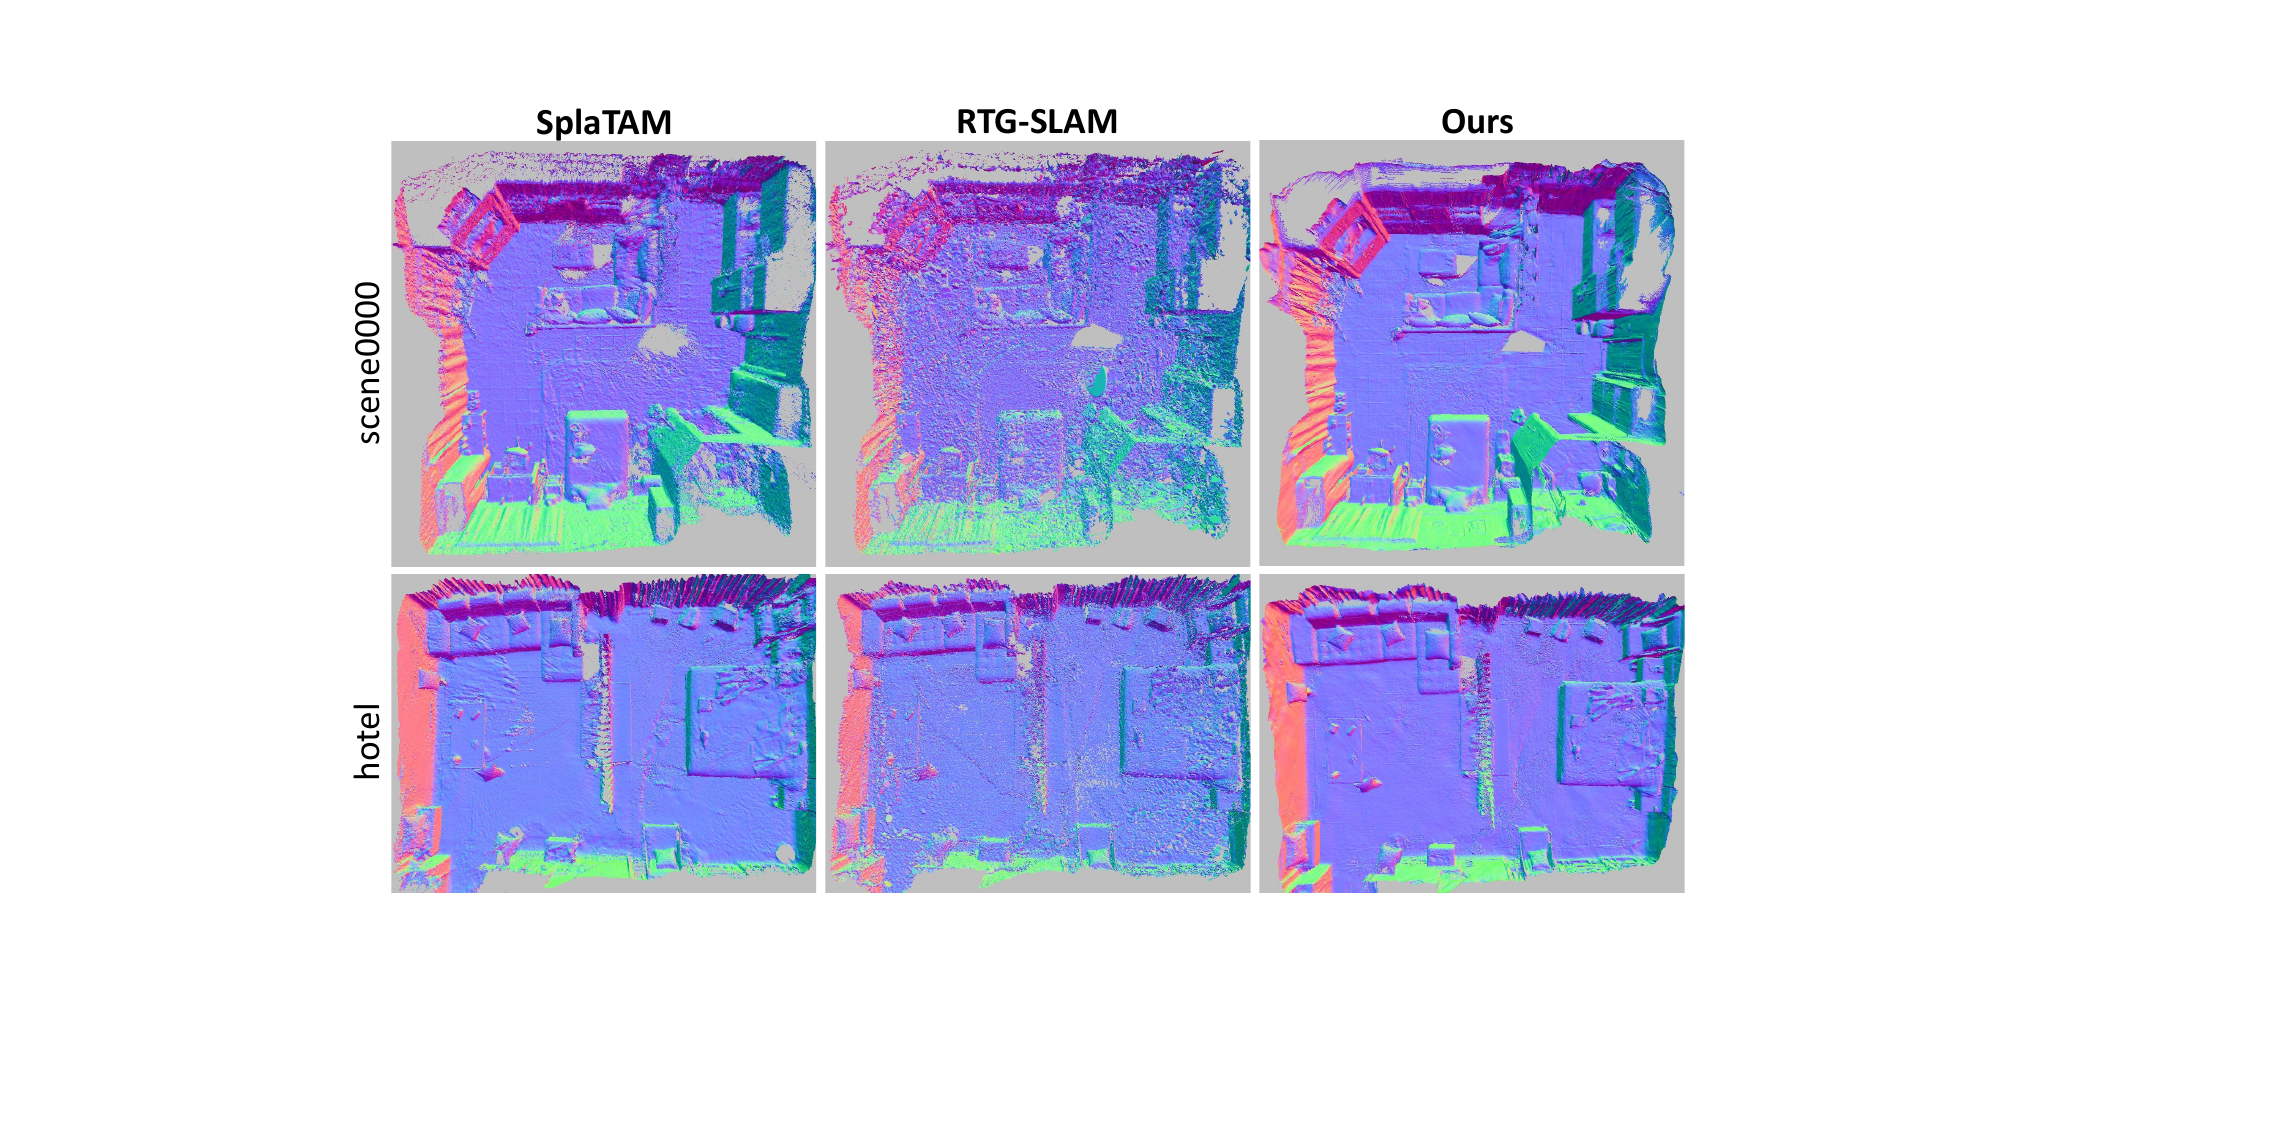}
  \end{center}
     \caption{ {Qualitative comparison of reconstruction results. In comparison to the previous methods, our reconstructions are smoother and contain
more details.
     }}
  \label{fig: mesh}
\end{figure}

\noindent
\textbf{Additional qualitative results on view rendering.}
{
    In this section, we provide rendering comparison results between SplaTAM \cite{splatam}, RTG-SAM \cite{rtg}, and our OG-Mapping across all input perspectives on hotel \cite{rtg} and scene0000 \cite{scannet} scenes. 
    The results are provided in the attached videos($hotel.mp4$ and $scene0000.mp4$). Notably, only SplaTAM utilizes all input perspectives for mapping, according to its default settings. 
    For RTG-SLAM and our method, some input perspectives are excluded from training for faster processing speed. 
    Additionally, we provide new perspective rendering video results on room0 \cite{replica} and scene0207 \cite{scannet}($novel\_view\_room0.mp4$ and $novel\_view\_scene0207.mp4$).
    The new viewpoint trajectories were generated by applying random Euler angle rotations of 25\textdegree to 35\textdegree and translation adjustments of 5 $cm$ to 10 $cm$ to the input viewpoint trajectories.
}

\begin{figure}[h]
  \begin{center}
  \includegraphics[width=1.0\linewidth]{./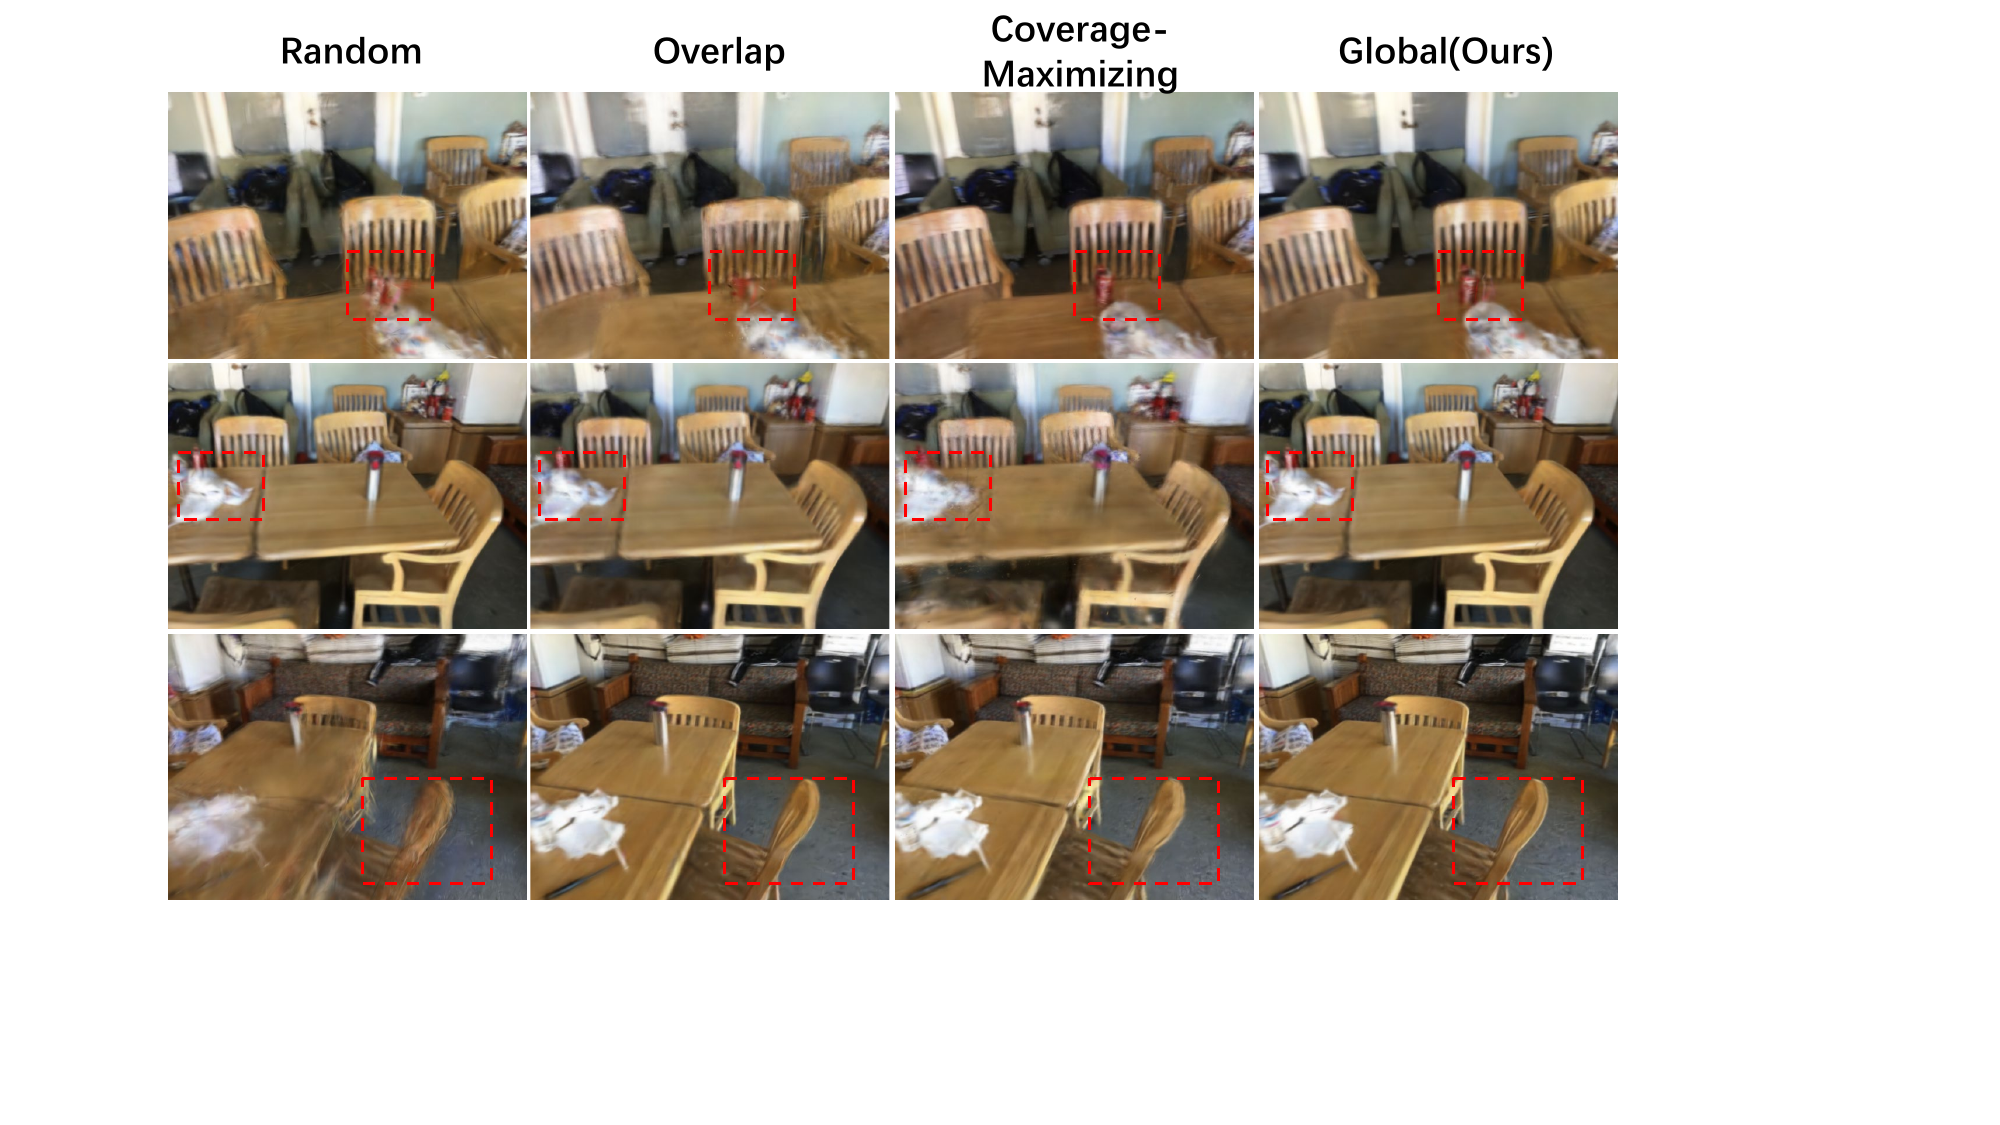}
  \end{center}
     \caption{ {Qualitative comparison of different keyframe window building method on $scene0059$ \cite{scannet}.}}
  \label{fig: keyframe_sup}
\end{figure}
\noindent
\textbf{Additional results on keyframe window building method.}
{
  The primary paper includes the results of ablation experiments on the keyframe window building method using the Replica dataset.
  In this section, we show more qualitative results from different views on real-world scene $scene0059$ \cite{scannet} in Fig. \ref{fig: keyframe_sup}.
  The quantitative results are shown in Tab. \ref{tab:keyframe_performance_comparison2}. 
  These fixed keyframe window methods are hindered by incorrect local optimization issues, which only ensure mapping quality within a specific area. In contrast, our dynamic keyframe window strategy can significantly improve the
  performance and the robustness of the reconstruction results.
}

}

\begin{figure*}[h]
  \begin{center}
  \includegraphics[width=0.98\linewidth]{./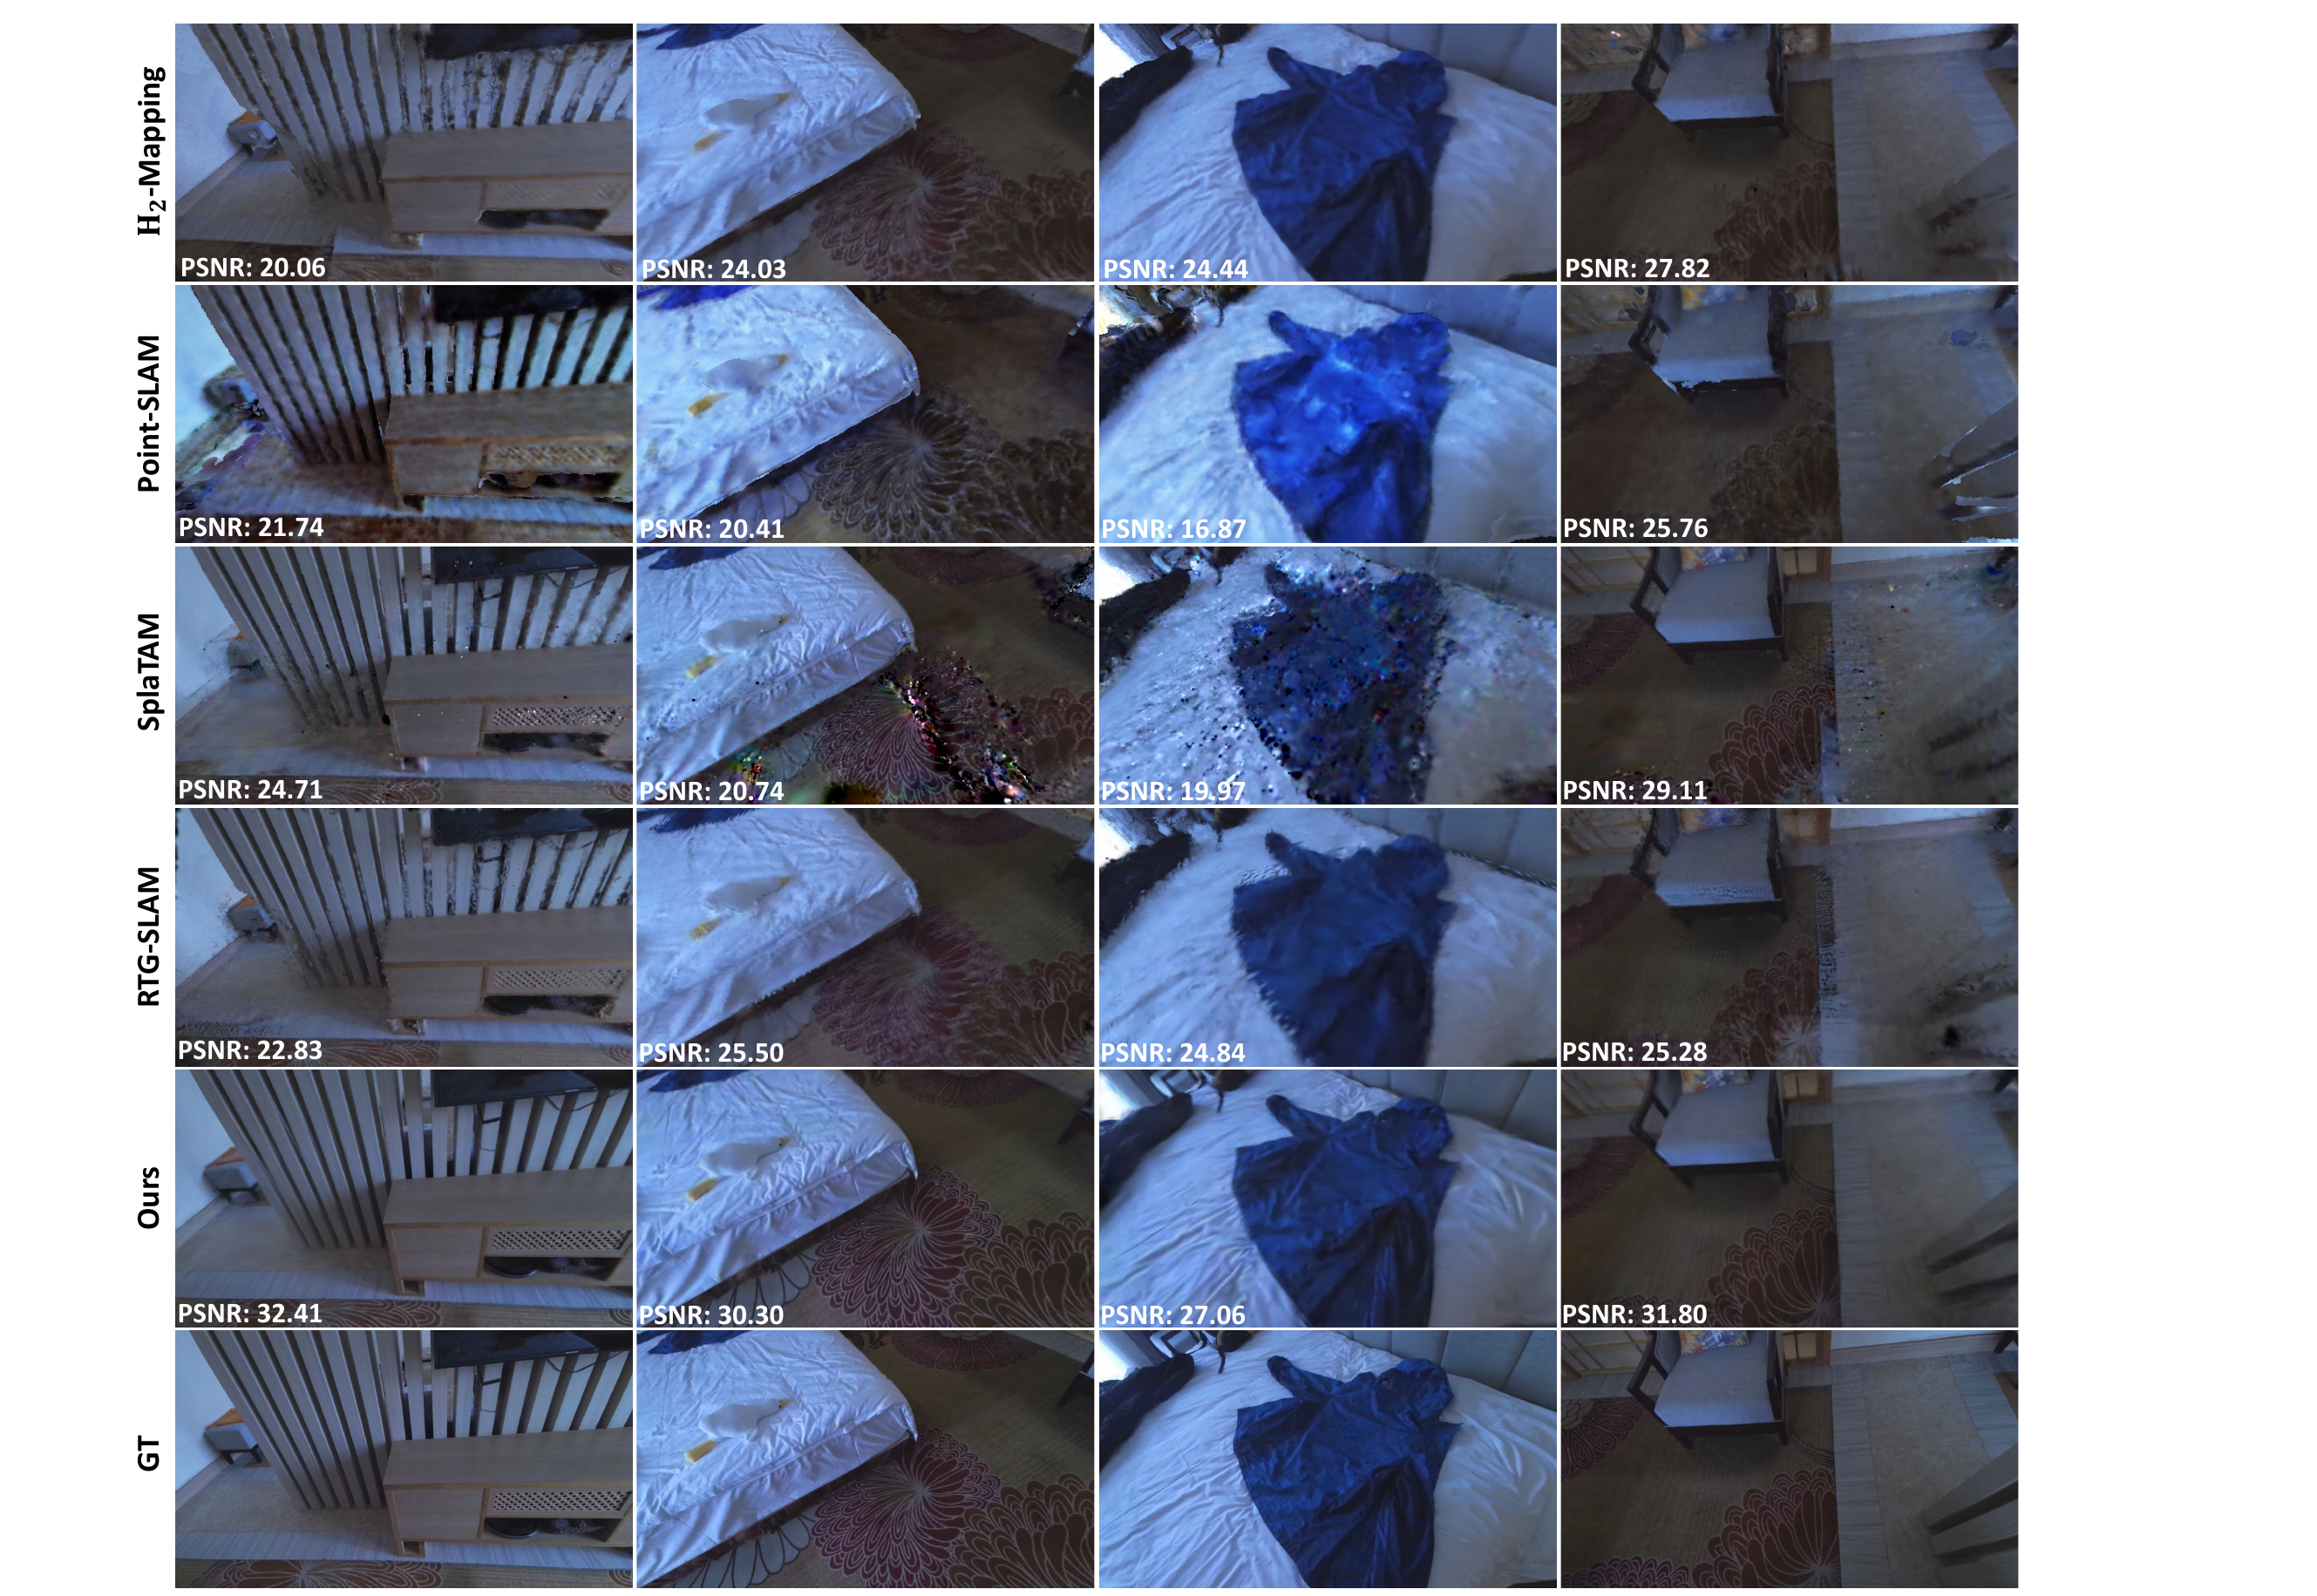}
  \end{center}
     \caption{ {Qualitative comparison of  training view rendering on the hotel dataset \cite{rtg}.
     The PSNR metric for current viewpoint is indicated in the lower left corner.}}
  \label{fig: hotel}
\end{figure*}
